# Supplementary material for: Learning Transferable 3D Adversarial Cloaks for Deep Trained Detectors
Source: arXiv:2104.11101 source file (2021-04-22)

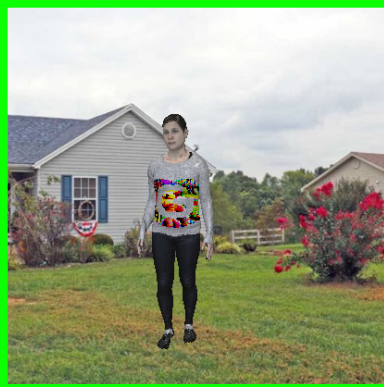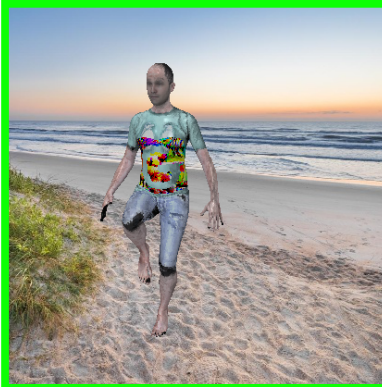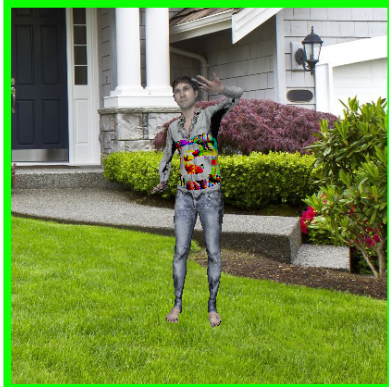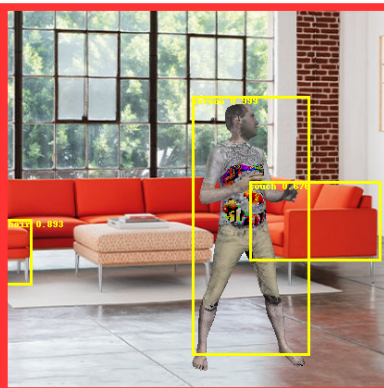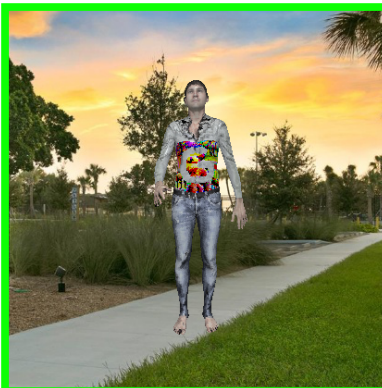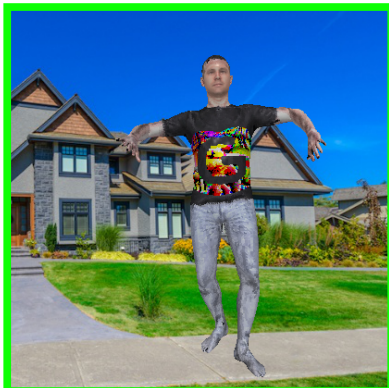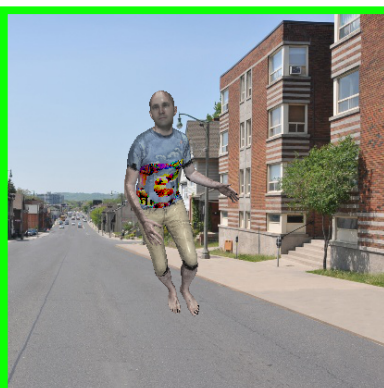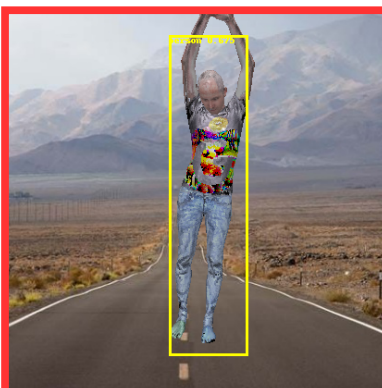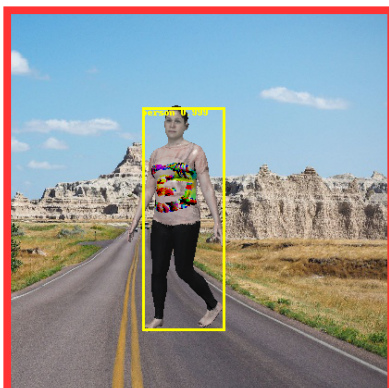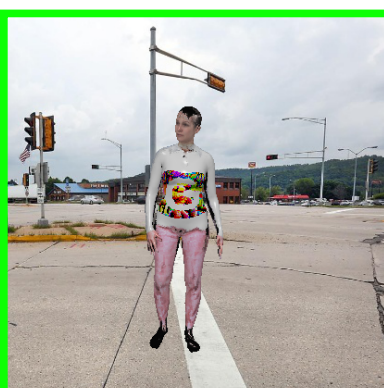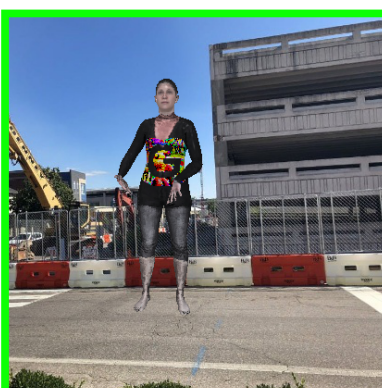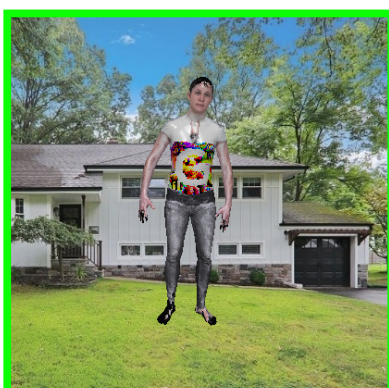

Supplement: Supplementary file 1 [file success_fail.pdf]
